# Supplementary material for: A Tactile Void
Source: arXiv:2412.04024 source file (2025-03-28)
Supplement: Supplementary file 1 [file SupMat.pdf]

# Supplementary Materials for : "A Tactile Void"

P. Tapie,[1] D. Barreiros Scatamburlo,[1] A. Chateauminois,[2] and E. Wandersman[1,*]

[1]*Laboratoire Jean Perrin, UMR 8237 Sorbonne Université/CNRS, Institut de Biologie Paris Seine, 4 Place Jussieu, F-75005 Paris, France*

[2]*Laboratoire Sciences et Ingénierie de la Matière Molle, UMR 7615 CNRS, ESPCI Paris, Université PSL, Sorbonne Université, F-75005 Paris, France*

(Dated: December 5, 2024)

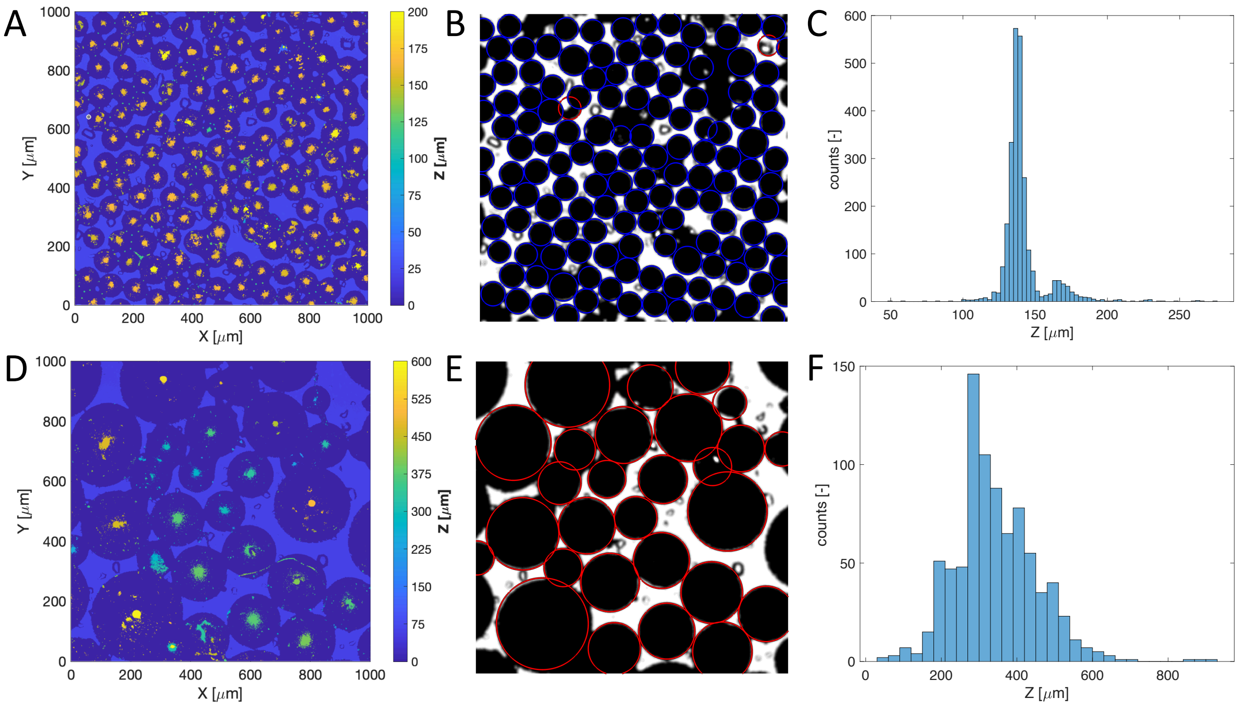


FIG. S1. For the rough- sample, A) Height field deduced from a profilometer measurement. The values 'zero' correspond to non-detected regions. B) Binarized image, over wich detected circles (blue) have been superimposed. Red circles are out-filtered structures. C) Histogram of the asperity heights, to which the glue base plane height has been subtracted. For the rough+ sample, D) Height field deduced from a profilometer measurement. E) Binarized image, over which detected and manually selected circles (red) have been superimposed. F) Histogram of the asperity heights, to which the glue base plane height has been subtracted.

## I. PROFILOMETRY AND ASPERITY HEIGHT DISTRIBUTION

We used an optical profilometer (Zegage Pro, Ametek inc, objective magnification x5) to measure the height distribution of our model rough surfaces. The profilometer can measure heights from interference patterns if the angle between the surface and the optical axis is less than 15°. Since our surfaces are made of polystyren or glass spheres glued on a glass plate, only the heights close to the spheres apexes can be measured, as well as the epoxy glue plane they are lying onto (see Fig. S1A for the rough- sample, Fig.S1D for the rough+ sample). For a given sphere, the non-detected region spans over its whole diameter for which the slopes are too large. Using a Hough Transform method on these non-detected

* elie.wandersman@sorbonne-universite.fr

regions (in practice the *imfindcircle function of Matlab*), we determined the positions and diameters of the spheres. Within each of these spheres, we measured the most probable height values and used it as its asperity height $z_i$. Profilometer measurements were repeated on different locations of the samples (N=20 for rough- yielding a total number of measured asperity heights $N_z^- \approx 2500$ on the one hand, and N=40 for rough+ yielding $N_z^+ \approx 900$ on the other hand.). Figures S1C and F present the histograms of the $z_i$ values obtained from these measurements, for the rough- and rough+ samples, respectively. The average height and standard deviation are respectivel 141±16 $\mu$m (resp. 325 ±128 $\mu$m).

## II. IMAGE ANALYSIS OF THE CAVITY

Image of the cavity are taken at 20 Hz in transmission. The images are binarized, holes are filled and we used the *regionprops function of Matlab* to detect the centroid of the cavity, and its edges. Moving to polar coordinates centered on the cavity centroid, we compute $r(\theta)$. The radius is interpolated on a theta grid ($\delta\theta = \pi/100$). For static normal contact, the radial displacement is defined as $u_r^N = r(\theta, F_N \neq 0) - r(\theta(F_N = 0)$. The radial displacement is well fitted by a $\cos(2\theta)$ function of amplitude $U_r^N$, but for computing time reasons, we preferred to compute the standard deviation of $u_r$, $\sigma_u$. The oscillation amplitude is then computed as $U_r^N = \sqrt{2}\sigma_u$. We checked that fitting or taking the standard deviation yielded similar results.

For friction sliding experiments, the radial displacement is computed by subtracting the profile at rest under the same normal force, prior to sliding: $u_r^S = r(\theta, F_N \neq 0, v \neq 0) - r(\theta, F_N \neq 0, v = 0)$.

To estimate the measurement noise, we performed out-of-contact experiments, displacing the rough plane at $v$=0.1 mm/s underneath the cylinder. Plots of the $x_c(t)$, $z_c(t)$ and $U_r^S(t)$ are shown on Fig.2. Taking the standard deviations of these signals as measurement noises $\sigma_{\delta x}$,$\sigma_{\delta z}$ and $\sigma_{\delta U}$, one finds after averaging over 15 different experiments, $\sigma_{\delta x}$= 0.39$\mu$m. $\sigma_{\delta z}$=0.17 $\mu$m and $\sigma_{\delta U}$= 0.06$\mu$m.

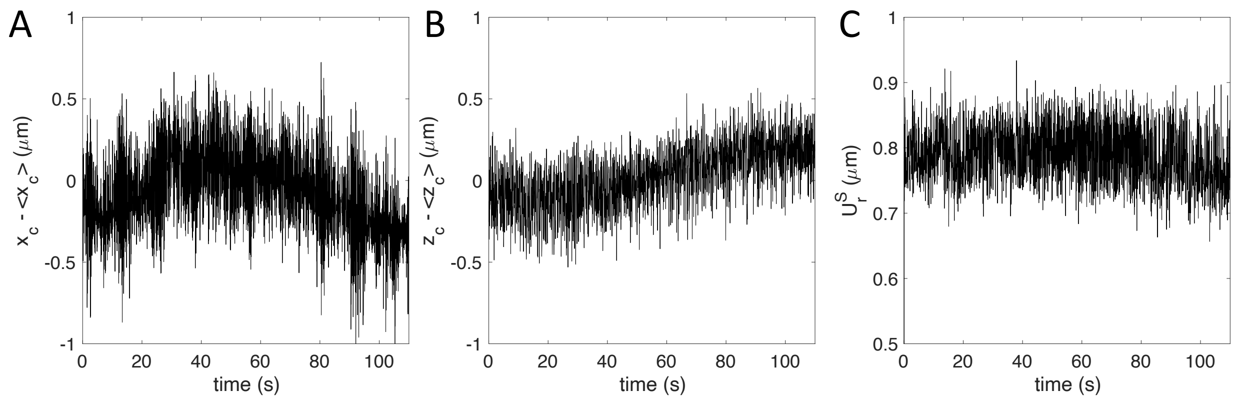


FIG. S2. Time traces of A) $x_c - < x_c >$, B) $z_c - < z_c >$ and C) $U_r^S$ for an out-of-contact experiment ($F_n = 0$, $v = 0.1$ mm/s).

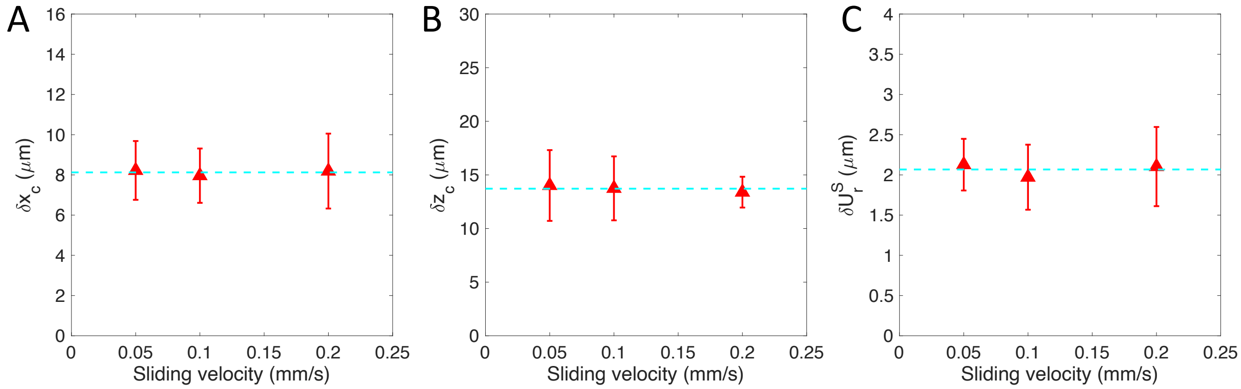


FIG. S3. A) Averaged fluctuations of the x-coordinate of the centroid, $\delta x_c$ at $F_n$=1N and different sliding velocities $v$. B) Same for the fluctuations of the z-coordinate of the centroid, $\delta z_c$ and C) for the radial displacement fluctuations $\delta U_r^S$.

## III. QUASI-STATICITY OF THE DYNAMICS AND DEFORMATION

We performed experiments at different sliding velocities ($v$, from 0.05 mm/s to 0.2 mm/s) to test the quasi-staticity of the cavity dynamics. On Fig. S3, we plot the averaged fluctuations of the cavity position and deformation, at the same normal force (here $F_n$=1 N), as a function of $v$. None of these quantities show a velocity dependence. The same behavior is observed at different normal forces. We conclude that the probed dynamics is independent of the sliding velocity.

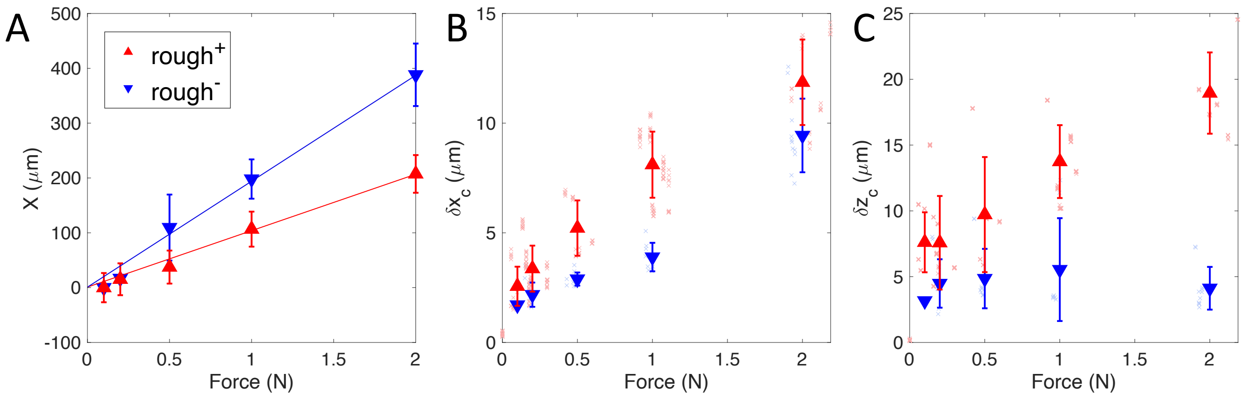


FIG. S4. A) Time-averaged $x_c$ displacement of the cavity centroid, as a function of the normal load. The lines are linear fits to the data. B) Standard deviation of $x_c$ displacement, $\delta$x. C) Standard deviation of $z_c$ displacement, $\delta$z.

## IV. FLUCTUATIONS AND POWER SPECTRUMS

On Fig. S4A and B we have plotted the average and standard deviation of the $x_c$ position as a function of the normal load, for both textures. We observe that the time-averaged $\bar{x}_c$ increase quasi-linearly with the normal force, with a slope respectively of 380 $\mu$m/N (resp 205 $\mu$m/N) for the rough- (rough+) surface, allowing to discriminate both textures. Noticeably, the magnitude of the time averaged lateral displacement $X$ of the cavity is correlated to the magnitude of the friction forces reported in Fig. 1D in the main text. Conversely, the fluctuations of $x_c$ on the contrary are not good texture discriminant. In the transverse $Z$ direction, fluctuations $\delta z_c$ are separated for rough- and rough+ samples. Typically, values of $\delta z_c$ are larger in amplitude than $\delta U_r^S$ fluctuations (Fig.3F, main text) but increase more moderately with the normal load.

What are the differences between the $\delta z_c$ and the $\delta U_r^S$ fluctuations ? On Fig. S5A we plot time traces of $z_c(v.t)$ and $U_r^S(v.t)$. Typically, the $z_c$ signal shows more large wavelength fluctuations than $\delta U_r^S$. This can be better evidenced by looking at the Power Spectrum of $z_c$ and $U_r^S$ fluctuations, as plotted on Fig.S5B (rough+) and C (rough-), as a function of the normalized wave vector $q.d$, $d$ being the particle diameter. Note that these spectrum have been normalized by the variance of the corresponding signal, to cancel their amplitude differences. The $z_c$ spectrum are found to decay as $q^{-2}$ over the whole wave vector range. The $U_r^S$ spectrum is quite comparable at low wave vectors, but present an excess of noise density

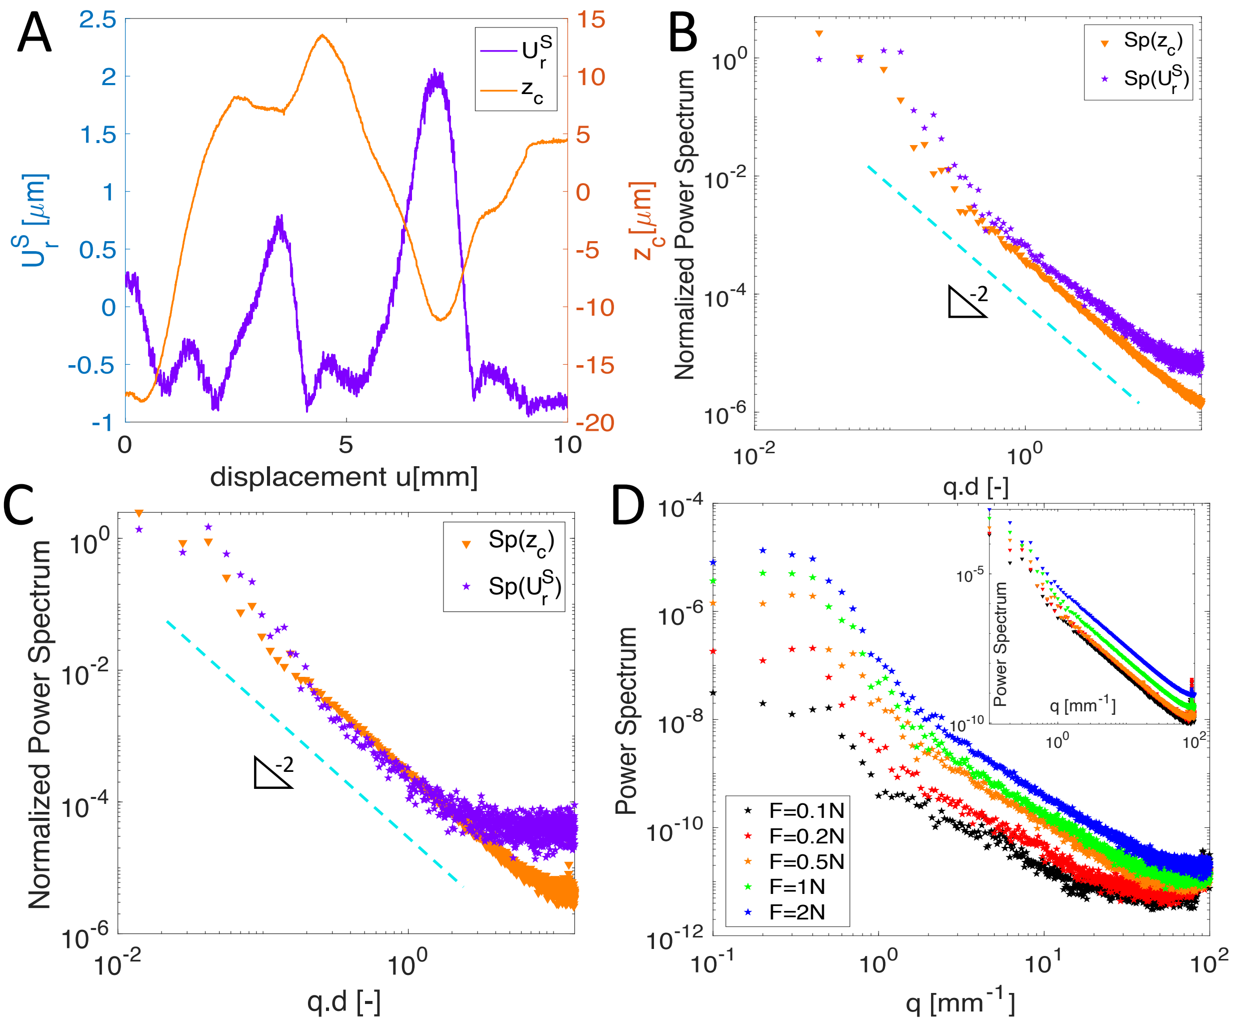


FIG. S5. A) Time traces of the $z_c$ displacement (orange, right scale) and $U_r^S$ (purple, left scale). The signal averages have been substracted. B) Normalized Power Spectrum of $z_c$ and $U_r^S$ as a function of the normalized wave vector $qd$, $d$ being the averaged particle diameter, for the rough+ sample, at $F_n$=0.5 N. C) Same for the rough- sample. D) Power Spectrum of the deformation $U_r^S$ for different normal load, for rough+ sample. Inset, Spectrum of $z_c$.

at larger wave vectors, with a cross-over at $q.d \sim 1$. It suggests that shape fluctuations are more sensitive to shorter length scale, close to the particle roughness length scale. We also found that the shape fluctuation spectrum is more sensitive to normal force variations than position fluctuations (Fig. S5D), since different spectra at different normal forces are more separated.
